# Supplementary material for: Publishing Neural Networks in Drug Discovery Might Compromise Training Data Privacy
Source: arXiv:2410.16975 ancillary file (2024-10-22)
Supplement: Supplementary file 1 [file Paper_Privacy_risks_Supplementary_Information.pdf]

# Publishing Neural Networks in Drug Discovery Compromises Training Data Privacy

A Preprint

**Fabian P. Krüger**[1,2,3] **Johan Östman**[4] **Lewis Mervin**[5] **Igor V. Tetko**[3] **Ola Engkvist**[1,6]

[1] **AstraZeneca R&D**
Discovery Sciences
Molecular AI
431 83 Mölndal, Sweden

[2] **Technical University of Munich**
TUM School of Computation,
Information and Technology
Department of Mathematics
80333 Munich, Germany

[3] **Helmholtz Munich**
Molecular Targets and Therapeutics Center
Institute of Structural Biology
85764 Neuherberg, Germany

[4] **AI Sweden**
41756 Gothenburg, Sweden

[5] **AstraZeneca R&D**
Discovery Sciences
Molecular AI
CB2 0AA Cambridge, UK

[6] **Chalmers University of Technology**
Department of Computer Science
and Engineering
412 96 Gothenburg, Sweden

## Supplementary information

### Derivation of the baseline TPR at an FPR of 0

In order to find the baseline for the TPR at FPR $= 0$, we calculate the expected value of the probability distribution for assigning memberships without any knowledge about the model. In our experiment, the adversary gets a training data sample with a probability of $\frac{2}{3}$ and a non-training data sample with a probability of $\frac{1}{3}$. For our baseline we chose to have our baseline built on knowing these probabilities, which is a rather conservative approach. Given that it is more likely that a molecule comes from the training data, our baseline adversary will always predict that it was part of the training data. Therefore, the probability distribution for the TPR at FPR $= 0$ is given by

$$P\left(\text{TPR} = \frac{k}{N}\right) = \left(\frac{2}{3}\right)^k \cdot \frac{1}{3}, \tag{1}$$

with $k$ being the number of true positives and $N$ the total number of positives (training data samples). We are interested in the expected value of this distribution:

$$\mathbb{E}[\text{TPR}] = \sum_{k=0}^{N} \frac{k}{N} \left(\frac{2}{3}\right)^k \cdot \frac{1}{3} \tag{2}$$

$$\mathbb{E}[\text{TPR}] = \frac{1}{3N} \sum_{k=0}^{N} k \left(\frac{2}{3}\right)^k \tag{3}$$

Since our number of training samples $N$ is very large (859 for our smallest dataset), this sum is very well approximated by taking the sum to infinity:

$$\mathbb{E}[\text{TPR}] \approx \frac{1}{3N} \sum_{k=0}^{\infty} k \left(\frac{2}{3}\right)^k \tag{4}$$

In order to find a computationally tractable solution for this expected value, we use the closed form of the geometric series:

$$\sum_{k=0}^{\infty} x^k = \frac{1}{1-x} \tag{5}$$

We differentiate both sides with respect to $x$:

$$\frac{d}{dx}\left(\frac{1}{1-x}\right) = \sum_{k=0}^{\infty} kx^{k-1} \tag{6}$$

$$\frac{1}{(1-x)^2} = \sum_{k=0}^{\infty} kx^{k-1} \tag{7}$$

Finally, we multiply both sides of the equation by $x$ to get our desired expression:

$$\frac{x}{(1-x)^2} = \sum_{k=0}^{\infty} kx^k \tag{8}$$

Substituting $x = \frac{2}{3}$:

$$\sum_{k=0}^{\infty} k \left(\frac{2}{3}\right)^k = \frac{\frac{2}{3}}{\left(1-\frac{2}{3}\right)^2} = 6 \tag{9}$$

With this solution, we can now calculate the expected TPR at FPR $= 0$:

$$\mathbb{E}[\text{TPR}] \approx \frac{1}{3N} \cdot 6 = \frac{2}{N} \tag{10}$$

This is the baseline for our TPR in our experiments. Significantly higher values show that it is possible to gather information about the training data from the neural network.

## Figures

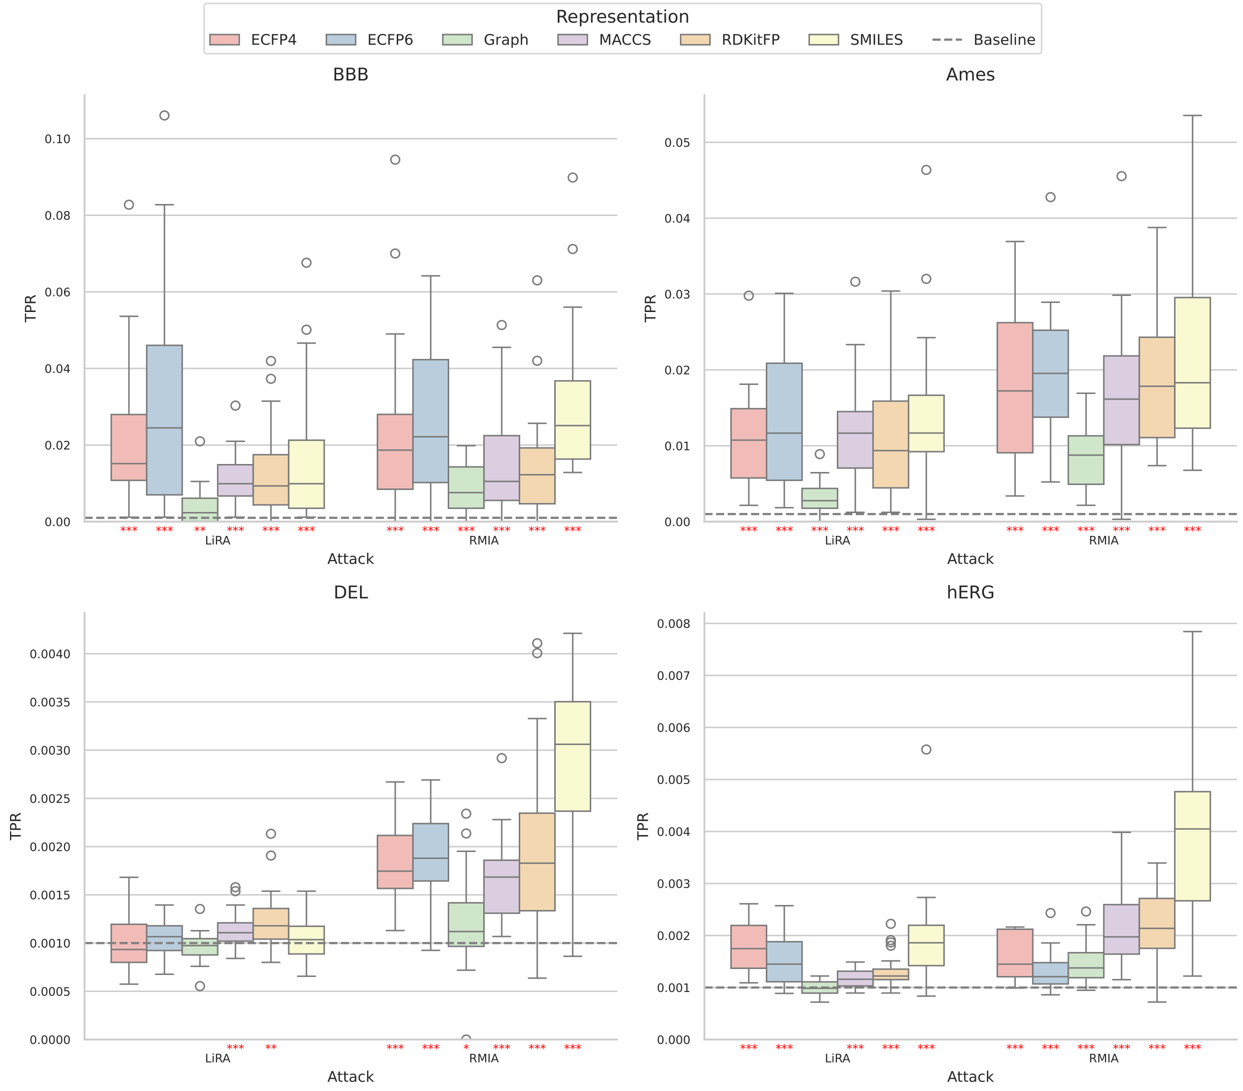


Figure 1: True positive rates for identifying training data molecules at a false positive rate of $10^{-3}$. The distributions of 20 experimental repetitions are shown for each representation and dataset, for both the likelihood ratio attack (LiRA) and the robust membership inference attack (RMIA). Distributions with significantly higher true positive rates than the baseline are indicated by red stars. A single star represents a p-value less than 0.05, two stars represent a p-value less than 0.01, and three stars represent a p-value less than 0.001. Training dataset sizes (total amount of positives) are: 859 molecules for the blood-brain barrier permeability dataset; 3,264 for the Ames mutagenicity prediction dataset; 48,837 for the DNA-encoded library enrichment dataset; and 137,853 for the hERG channel inhibition dataset.

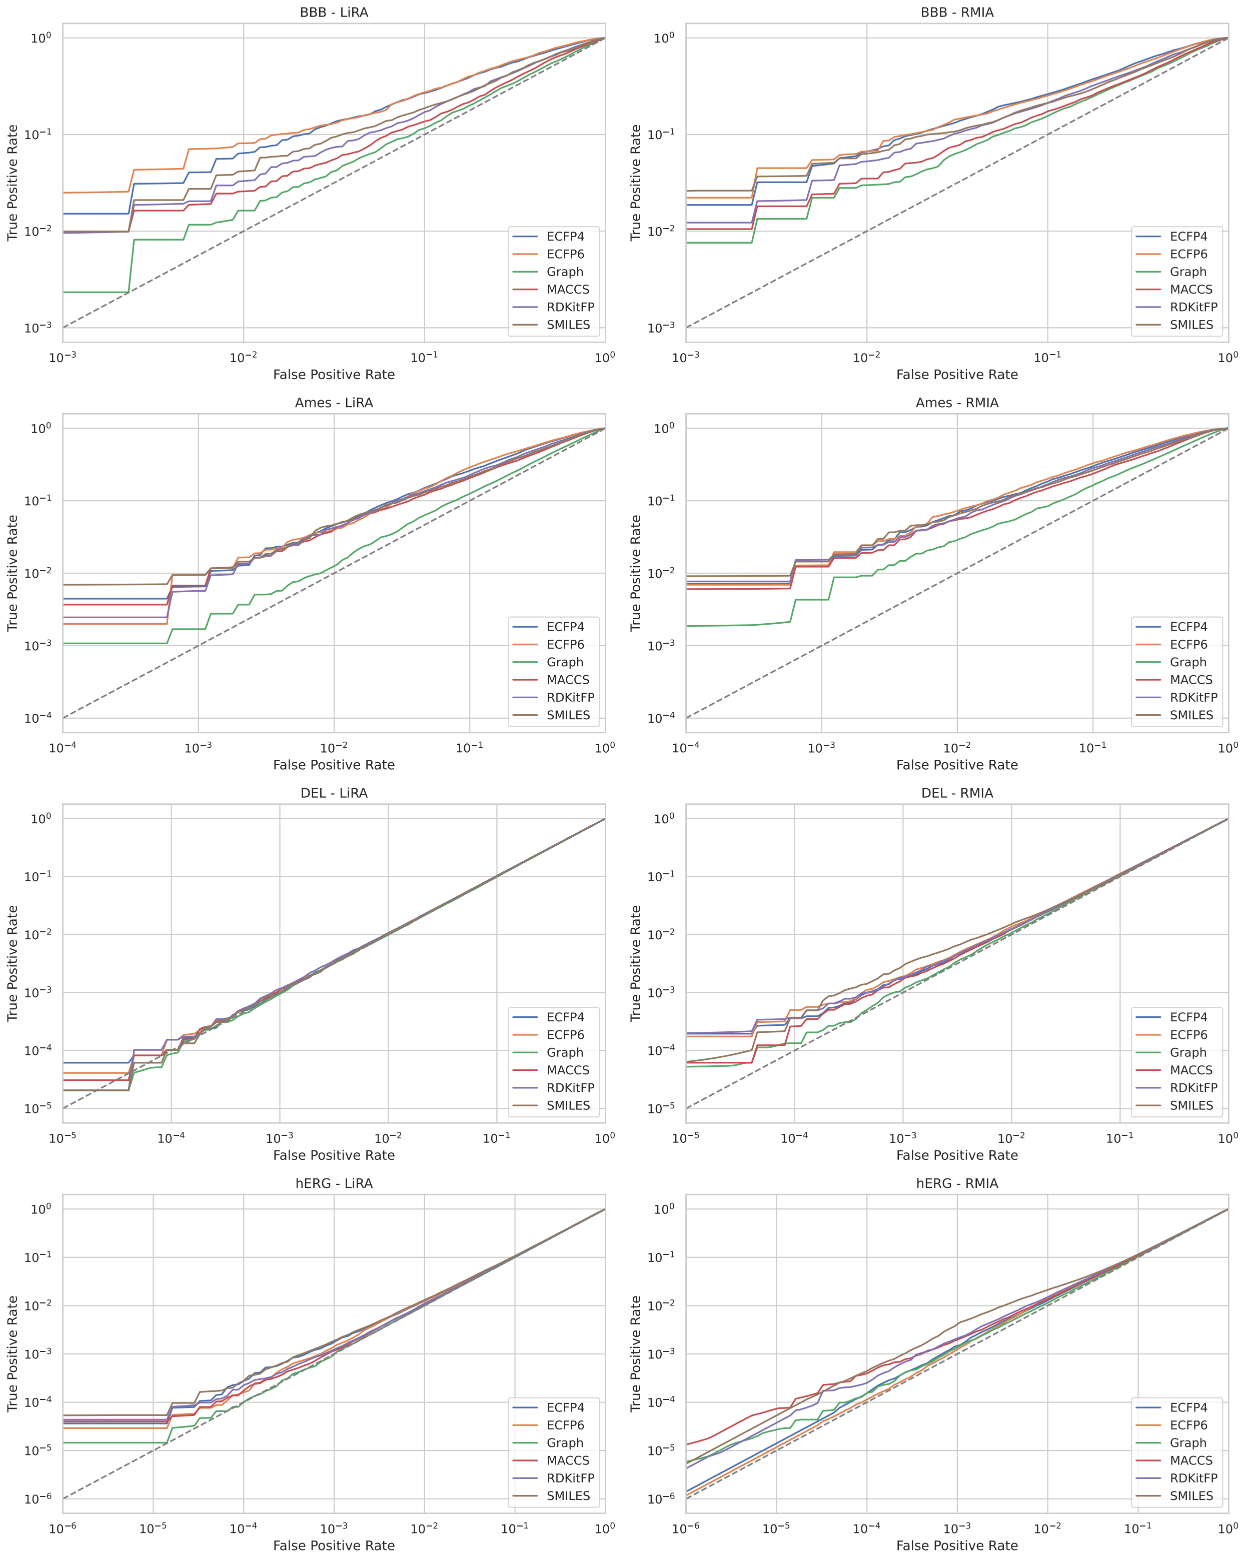


Figure 2: ROC curves for identifying training data molecules. Results are displayed for both the likelihood ratio attack (LiRA) and the robust membership inference attack (RMIA). The dashed line indicates the performance of random guessing. Training dataset sizes are: 859 molecules for the blood-brain barrier permeability dataset; 3,264 for the Ames mutagenicity prediction dataset; 48,837 for the DNA-encoded library enrichment dataset; and 137,853 for the hERG channel inhibition dataset.

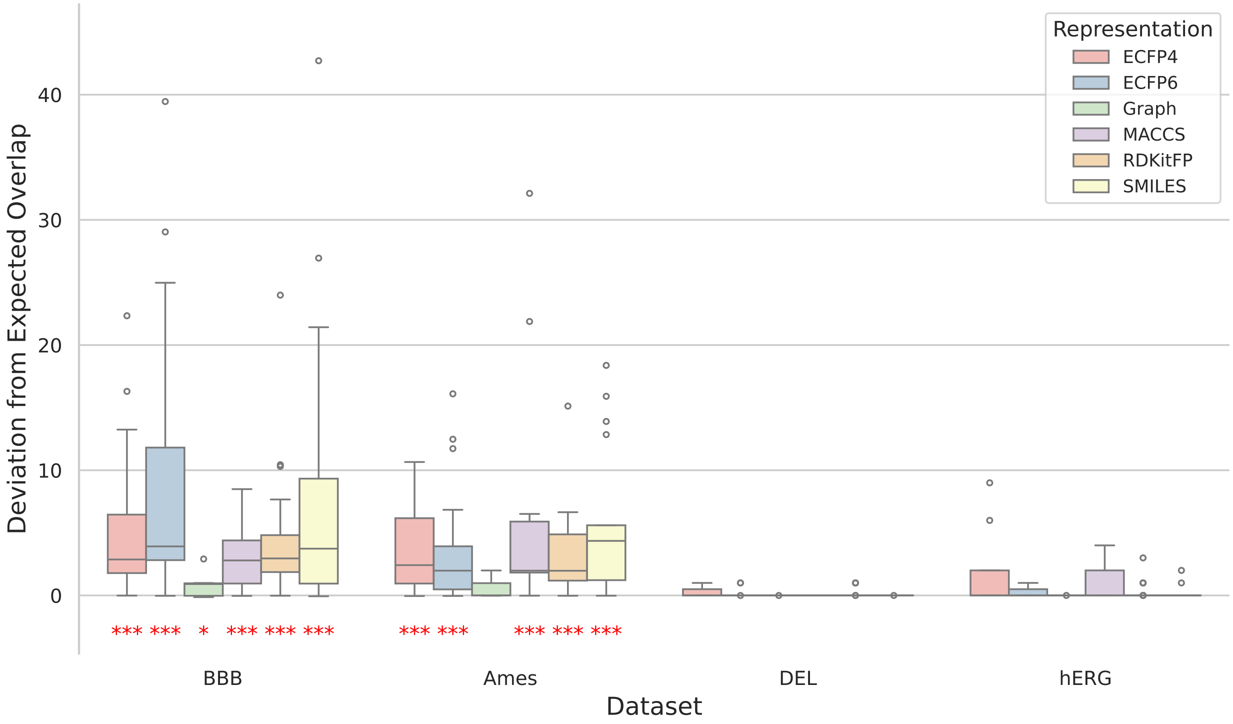


Figure 3: Deviations from the expected overlap of uncorrelated attacks. For each of our 20 experiment repetitions, we calculated the amount of molecules that were identified by both the likelihood ratio attack (LiRA) and the robust membership inference attack (RMIA) for each dataset and representation. We also calculated how many molecules would have been identified by both attacks if they were completely uncorrelated. This amount depended on the sizes of the sets of the identified molecules in each repetition. The figure shows the distribution of deviations from the expected overlap (for uncorrelated attacks) to the observed overlap. Distributions significantly greater than 0 are marked with red stars. A single star represents a p-value less than 0.05, two stars represent a p-value less than 0.01, and three stars represent a p-value less than 0.001.

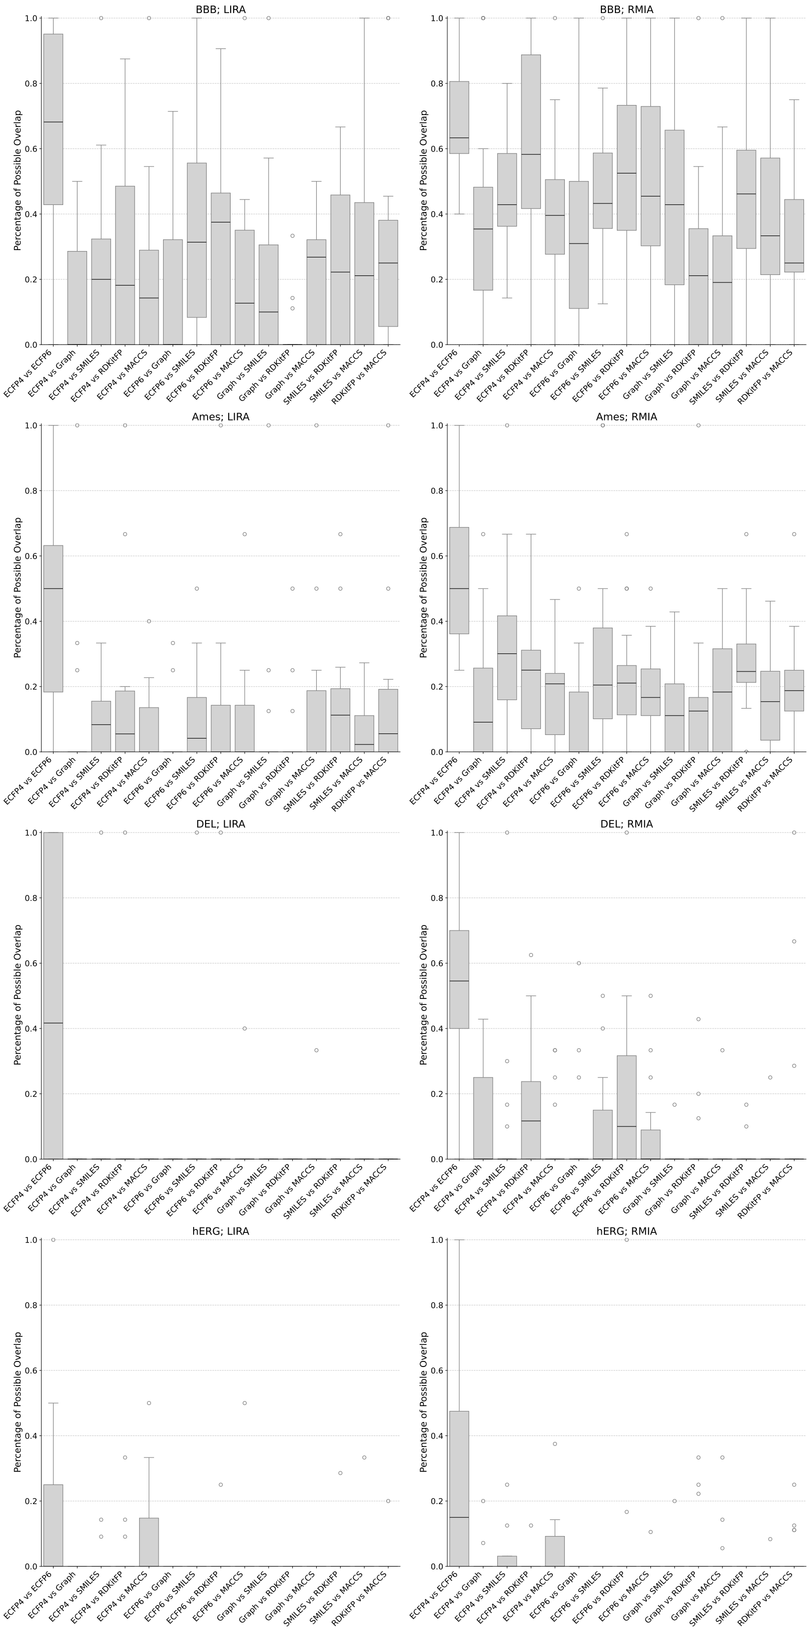


Figure 4: Overlap of identified molecules between models trained on different molecular representations of the same training data. The distribution displays the amount of overlap in our 20 experiment repetitions.

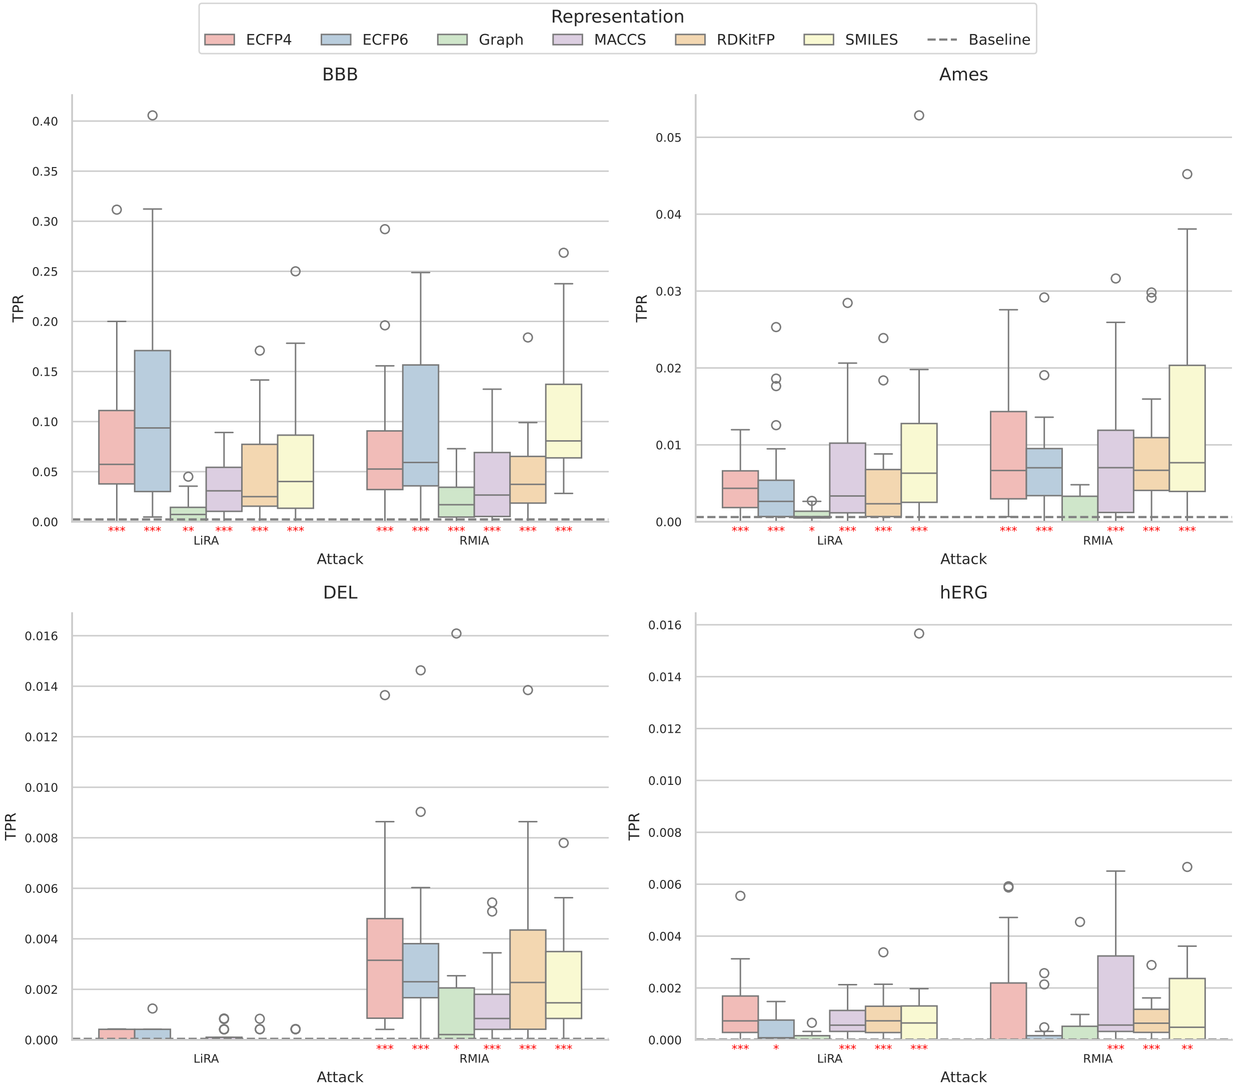


Figure 5: True positive rates for identifying training data molecules of the minority class at a false positive rate of 0. The distributions of 20 experimental repetitions are shown for each representation and dataset, for both the likelihood ratio attack (LiRA) and the robust membership inference attack (RMIA). The baseline for each dataset is 2 divided by the amount of minority class molecules in the training data. Distributions with significantly higher true positive rates are indicated by red stars. A single star represents a p-value less than 0.05, two stars represent a p-value less than 0.01, and three stars represent a p-value less than 0.001.

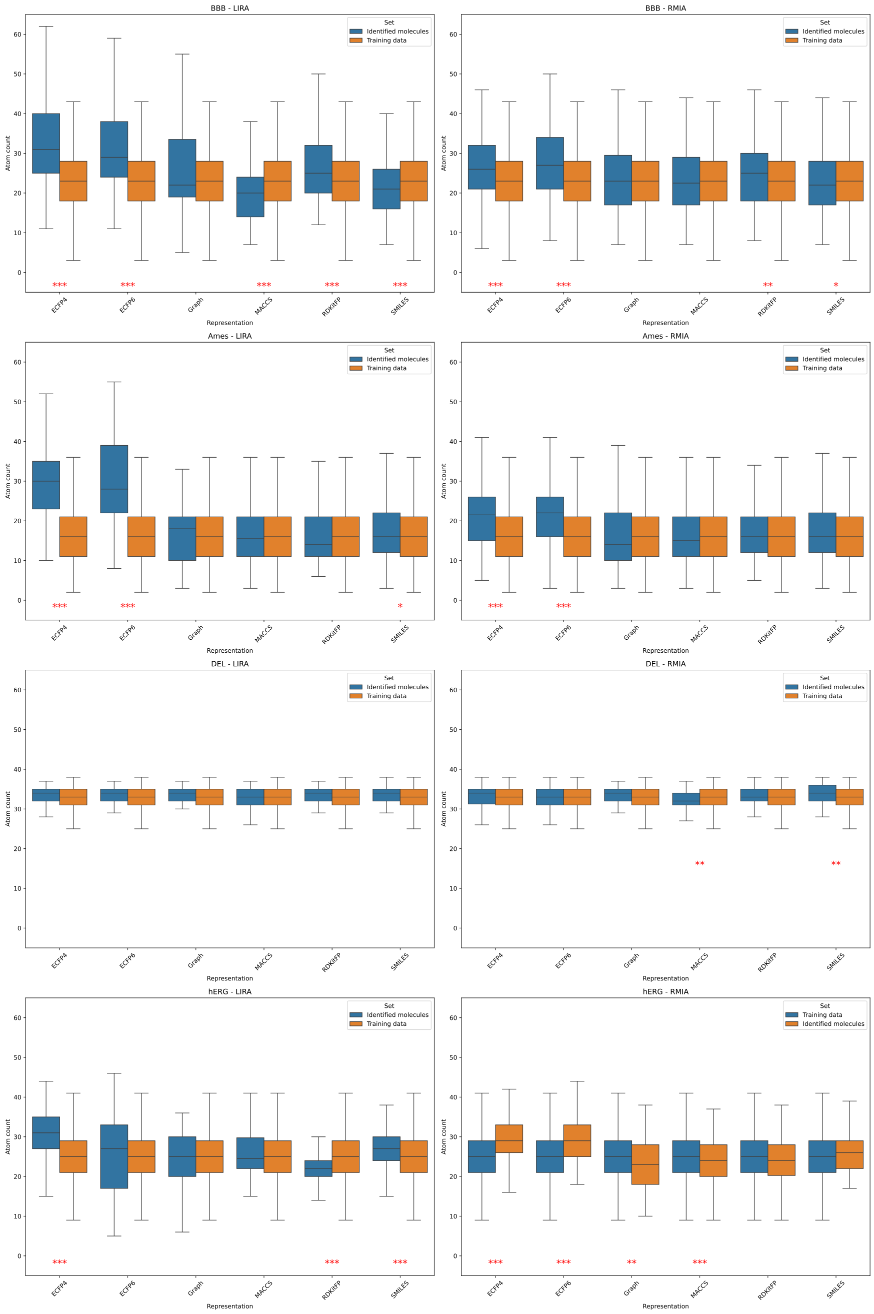


Figure 6: Distributions of molecular sizes, in terms of atom counts, are shown for the chemical structures identified at an FPR of 0 and for the corresponding training data. The data represents the aggregated results from 20 experimental repetitions. Significant differences between distributions are marked with red stars: one star for a p-value less than 0.05, two stars for a p-value less than 0.01, and three stars for a p-value less than 0.001.

## Tables

Table 1: Hyperparameter search spaces for MLP, MPNN, and CNN models.

| Model | Hyperparameter | Range |
|---|---|---|
| MLP | Dropout | 0.0 – 1.0 |
| | Hidden Dimension | 10 – 1000 |
| | Number of Hidden Layers | 1 – 5 |
| | Learning Rate | 1e-5 – 1e-2 |
| | Weight Decay | 1e-6 – 1e-3 |
| MPNN | Message Passing Steps | 2 – 6 |
| | Encoder Dropout | 0.0 – 0.4 |
| | Encoder Hidden Size | 300 – 2400 |
| | Bias in Encoder Layers | {True, False} |
| | Aggregation Method | {mean, sum, norm} |
| | Classifier Number of Hidden Layers | 1 – 3 |
| | Classifier Hidden Dimension | 300 – 2400 |
| | Classifier Dropout | 0.0 – 0.4 |
| | Learning Rate | 1e-5 – 1e-2 |
| | Weight Decay | 1e-6 – 1e-3 |
| CNN | Dropout | 0.0 – 1.0 |
| | Learning Rate | 1e-5 – 1e-2 |
| | Weight Decay | 1e-6 – 1e-3 |
